# Supplementary material for: A Systematic Study of Noise Effects in Hybrid Quantum-Classical Machine Learning
Source: arXiv:2604.11541 source file (2026-04-13)
Supplement: Supplementary file 1 [file appendix.tex]

\begin{appendix}
\section*{Complete Loss Curves and Accuracy Plots}
\label{app:all_plots}

This appendix presents the complete set of loss convergence curves and training--testing accuracy bar charts for all evaluated combinations of dataset-level noise, encoding-level (angle-space) noise, and circuit-level quantum noise. The corresponding visualizations are provided in Figs.~\ref{fig:loss_nods_grouped}--\ref{fig:acc_Random_grouped}.

For each dataset noise condition, figures are grouped by angle-space noise magnitude ($\sigma \in \{0, 0.01, 0.03, 0.05\}$). Within each subplot, loss curves correspond to all sixteen circuit-level noise configurations (see Figs.~\ref{fig:loss_nods_grouped}, \ref{fig:loss_gauss_grouped}, \ref{fig:loss_snp_grouped}, \ref{fig:loss_unif_grouped}, \ref{fig:loss_spec_grouped}, \ref{fig:loss_FD_grouped}, \ref{fig:loss_Quant_grouped}, and \ref{fig:loss_Random_grouped}), enabling direct comparison of optimization stability and convergence behavior under increasing noise severity.

The accompanying accuracy bar plots summarize the final training and testing accuracies for the same configurations (see Figs.~\ref{fig:acc_nods_grouped}, \ref{fig:acc_gauss_grouped}, \ref{fig:acc_snp_grouped}, \ref{fig:acc_unif_grouped}, \ref{fig:acc_spec_grouped}, \ref{fig:acc_FD_grouped}, \ref{fig:acc_Quant_grouped}, and \ref{fig:acc_Random_grouped}), facilitating analysis of generalization behavior and the relative impact of coherent versus incoherent noise sources.

Collectively, these visualizations corroborate the key findings discussed in the main text: abrupt optimization collapse under circuit-level quantum noise, gradual performance degradation under angle-space perturbations, and comparatively weaker sensitivity to dataset-level noise in the absence of hardware noise.

%-----------------------------------------%
% -----------No Dataset Noise-------------%
%-----------------------------------------%

\begin{figure*}[t]
    \centering

    \begin{subfigure}[t]{\linewidth}
        \centering
        \includegraphics[width=0.75\linewidth]{PaperSection/Pictures/PlotsAndGraphs/NoDSNoise/LossCurves_No Dataset Noise_No Angle Noise.pdf}
        \caption{Angle-space noise $\sigma = 0$}
        \label{fig:loss_nods_sigma_0}
    \end{subfigure}
    \hfill
    \begin{subfigure}[t]{\linewidth}
        \centering
        \includegraphics[width=0.75\linewidth]{PaperSection/Pictures/PlotsAndGraphs/NoDSNoise/LossCurves_No Dataset Noise_AngleSpaceNoiseSigma1.pdf}
        \caption{Angle-space noise $\sigma = 0.01$}
        \label{fig:loss_nods_sigma_001}
    \end{subfigure}

    \vspace{0.6em}

    \begin{subfigure}[t]{\linewidth}
        \centering
        \includegraphics[width=0.75\linewidth]{PaperSection/Pictures/PlotsAndGraphs/NoDSNoise/LossCurves_No Dataset Noise_AngleSpaceNoiseSigma3.pdf}
        \caption{Angle-space noise $\sigma = 0.03$}
        \label{fig:loss_nods_sigma_003}
    \end{subfigure}
    \hfill
    \begin{subfigure}[t]{\linewidth}
        \centering
        \includegraphics[width=0.75\linewidth]{PaperSection/Pictures/PlotsAndGraphs/NoDSNoise/LossCurves_No Dataset Noise_AngleSpaceNoiseSigma5.pdf}
        \caption{Angle-space noise $\sigma = 0.05$}
        \label{fig:loss_nods_sigma_005}
    \end{subfigure}

    \caption{Loss convergence curves for all circuit-level noise configurations under \textbf{no dataset noise}, shown for increasing angle-space noise magnitudes.}
    \label{fig:loss_nods_grouped}
\end{figure*}

\begin{figure*}[t]
    \centering

    \begin{subfigure}[t]{0.9\linewidth}
        \centering
        \includegraphics[width=0.8\linewidth]{PaperSection/Pictures/PlotsAndGraphs/NoDSNoise/AccuracyBars_No Dataset Noise_No Angle Noise.pdf}
        \caption{Angle-space noise $\sigma = 0$}
        \label{fig:acc_nods_sigma_0}
    \end{subfigure}
    \hfill
    \begin{subfigure}[t]{0.9\linewidth}
        \centering
        \includegraphics[width=0.8\linewidth]{PaperSection/Pictures/PlotsAndGraphs/NoDSNoise/AccuracyBars_No Dataset Noise_AngleSpaceNoiseSigma1.pdf}
        \caption{Angle-space noise $\sigma = 0.01$}
        \label{fig:acc_nods_sigma_001}
    \end{subfigure}

    \vspace{0.6em}

    \begin{subfigure}[t]{0.9\linewidth}
        \centering
        \includegraphics[width=0.8\linewidth]{PaperSection/Pictures/PlotsAndGraphs/NoDSNoise/AccuracyBars_No Dataset Noise_AngleSpaceNoiseSigma3.pdf}
        \caption{Angle-space noise $\sigma = 0.03$}
        \label{fig:acc_nods_sigma_003}
    \end{subfigure}
    \hfill
    \begin{subfigure}[t]{0.9\linewidth}
        \centering
        \includegraphics[width=0.8\linewidth]{PaperSection/Pictures/PlotsAndGraphs/NoDSNoise/AccuracyBars_No Dataset Noise_AngleSpaceNoiseSigma5.pdf}
        \caption{Angle-space noise $\sigma = 0.05$}
        \label{fig:acc_nods_sigma_005}
    \end{subfigure}

    \caption{Training and testing accuracy comparison for all circuit-level noise configurations under \textbf{no dataset noise}, shown for increasing angle-space perturbations.}
    \label{fig:acc_nods_grouped}
\end{figure*}
%----------------------------------------------------%
% -----------Gaussian Noise: Loss Curves-------------%
%----------------------------------------------------%

\begin{figure*}[t]
    \centering

    \begin{subfigure}[t]{0.9\linewidth}
        \centering
        \includegraphics[width=\linewidth]{PaperSection/Pictures/PlotsAndGraphs/GaussianNoise/LossCurves_Gaussian Noise_0.pdf}
        \caption{Angle-space noise $\sigma = 0$}
        \label{fig:loss_gauss_sigma_0}
    \end{subfigure}
    \hfill
    \begin{subfigure}[t]{0.9\linewidth}
        \centering
        \includegraphics[width=\linewidth]{PaperSection/Pictures/PlotsAndGraphs/GaussianNoise/LossCurves_Gaussian Noise_0.01.pdf}
        \caption{Angle-space noise $\sigma = 0.01$}
        \label{fig:loss_gauss_sigma_001}
    \end{subfigure}

    \vspace{0.6em}

    \begin{subfigure}[t]{0.9\linewidth}
        \centering
        \includegraphics[width=\linewidth]{PaperSection/Pictures/PlotsAndGraphs/GaussianNoise/LossCurves_Gaussian Noise_0.03.pdf}
        \caption{Angle-space noise $\sigma = 0.03$}
        \label{fig:loss_gauss_sigma_003}
    \end{subfigure}
    \hfill
    \begin{subfigure}[t]{0.9\linewidth}
        \centering
        \includegraphics[width=\linewidth]{PaperSection/Pictures/PlotsAndGraphs/GaussianNoise/LossCurves_Gaussian Noise_0.05.pdf}
        \caption{Angle-space noise $\sigma = 0.05$}
        \label{fig:loss_gauss_sigma_005}
    \end{subfigure}

    \caption{Loss convergence curves for all circuit-level noise configurations under \textbf{Gaussian dataset noise}, shown for increasing angle-space noise magnitudes.}
    \label{fig:loss_gauss_grouped}
\end{figure*}
%----------------------------------------------------%
% -----------Gaussian Noise: Accuracy Plots----------%
%----------------------------------------------------%

\begin{figure*}[t]
    \centering

    \begin{subfigure}[t]{0.9\linewidth}
        \centering
        \includegraphics[width=0.8\linewidth]{PaperSection/Pictures/PlotsAndGraphs/GaussianNoise/AccuracyBars_Gaussian Noise_0.pdf}
        \caption{Angle-space noise $\sigma = 0$}
        \label{fig:acc_gauss_sigma_0}
    \end{subfigure}
    \hfill
    \begin{subfigure}[t]{0.9\linewidth}
        \centering
        \includegraphics[width=0.8\linewidth]{PaperSection/Pictures/PlotsAndGraphs/GaussianNoise/AccuracyBars_Gaussian Noise_0.01.pdf}
        \caption{Angle-space noise $\sigma = 0.01$}
        \label{fig:acc_gauss_sigma_001}
    \end{subfigure}

    \vspace{0.6em}

    \begin{subfigure}[t]{0.9\linewidth}
        \centering
        \includegraphics[width=0.8\linewidth]{PaperSection/Pictures/PlotsAndGraphs/GaussianNoise/AccuracyBars_Gaussian Noise_0.03.pdf}
        \caption{Angle-space noise $\sigma = 0.03$}
        \label{fig:acc_gauss_sigma_003}
    \end{subfigure}
    \hfill
    \begin{subfigure}[t]{0.9\linewidth}
        \centering
        \includegraphics[width=0.8\linewidth]{PaperSection/Pictures/PlotsAndGraphs/GaussianNoise/AccuracyBars_Gaussian Noise_0.05.pdf}
        \caption{Angle-space noise $\sigma = 0.05$}
        \label{fig:acc_gauss_sigma_005}
    \end{subfigure}

    \caption{Training and testing accuracy comparison for all circuit-level noise configurations under \textbf{Gaussian dataset noise}, shown for increasing angle-space perturbations.}
    \label{fig:acc_gauss_grouped}
\end{figure*}
%------------------------------------------------------------%
% -----------Salt-and-Pepper Noise: Loss Curves--------------%
%------------------------------------------------------------%

\begin{figure*}[t]
    \centering

    \begin{subfigure}[t]{0.9\linewidth}
        \centering
        \includegraphics[width=\linewidth]{PaperSection/Pictures/PlotsAndGraphs/SaltAndPepperNoise/LossCurves_SaltNPepperNoise_0.pdf}
        \caption{Angle-space noise $\sigma = 0$}
        \label{fig:loss_snp_sigma_0}
    \end{subfigure}
    \hfill
    \begin{subfigure}[t]{0.9\linewidth}
        \centering
        \includegraphics[width=\linewidth]{PaperSection/Pictures/PlotsAndGraphs/SaltAndPepperNoise/LossCurves_SaltNPepperNoise_0.01.pdf}
        \caption{Angle-space noise $\sigma = 0.01$}
        \label{fig:loss_snp_sigma_001}
    \end{subfigure}

    \vspace{0.6em}

    \begin{subfigure}[t]{0.9\linewidth}
        \centering
        \includegraphics[width=\linewidth]{PaperSection/Pictures/PlotsAndGraphs/SaltAndPepperNoise/LossCurves_SaltNPepperNoise_0.03.pdf}
        \caption{Angle-space noise $\sigma = 0.03$}
        \label{fig:loss_snp_sigma_003}
    \end{subfigure}
    \hfill
    \begin{subfigure}[t]{0.9\linewidth}
        \centering
        \includegraphics[width=\linewidth]{PaperSection/Pictures/PlotsAndGraphs/SaltAndPepperNoise/LossCurves_SaltNPepperNoise_0.05.pdf}
        \caption{Angle-space noise $\sigma = 0.05$}
        \label{fig:loss_snp_sigma_005}
    \end{subfigure}

    \caption{Loss convergence curves for all circuit-level noise configurations under \textbf{salt-and-pepper (impulse) dataset noise}, shown for increasing angle-space noise magnitudes.}
    \label{fig:loss_snp_grouped}
\end{figure*}
%------------------------------------------------------------%
% -----------Salt-and-Pepper Noise: Accuracy Plots------------%
%------------------------------------------------------------%

\begin{figure*}[t]
    \centering

    \begin{subfigure}[t]{0.9\linewidth}
        \centering
        \includegraphics[width=0.8\linewidth]{PaperSection/Pictures/PlotsAndGraphs/SaltAndPepperNoise/AccuracyBars_SaltNPepperNoise_0.pdf}
        \caption{Angle-space noise $\sigma = 0$}
        \label{fig:acc_snp_sigma_0}
    \end{subfigure}
    \hfill
    \begin{subfigure}[t]{0.9\linewidth}
        \centering
        \includegraphics[width=0.8\linewidth]{PaperSection/Pictures/PlotsAndGraphs/SaltAndPepperNoise/AccuracyBars_SaltNPepperNoise_0.01.pdf}
        \caption{Angle-space noise $\sigma = 0.01$}
        \label{fig:acc_snp_sigma_001}
    \end{subfigure}

    \vspace{0.6em}

    \begin{subfigure}[t]{0.9\linewidth}
        \centering
        \includegraphics[width=0.8\linewidth]{PaperSection/Pictures/PlotsAndGraphs/SaltAndPepperNoise/AccuracyBars_SaltNPepperNoise_0.03.pdf}
        \caption{Angle-space noise $\sigma = 0.03$}
        \label{fig:acc_snp_sigma_003}
    \end{subfigure}
    \hfill
    \begin{subfigure}[t]{0.9\linewidth}
        \centering
        \includegraphics[width=0.8\linewidth]{PaperSection/Pictures/PlotsAndGraphs/SaltAndPepperNoise/AccuracyBars_SaltNPepperNoise_0.05.pdf}
        \caption{Angle-space noise $\sigma = 0.05$}
        \label{fig:acc_snp_sigma_005}
    \end{subfigure}

    \caption{Training and testing accuracy comparison for all circuit-level noise configurations under \textbf{salt-and-pepper (impulse) dataset noise}, shown for increasing angle-space perturbations.}
    \label{fig:acc_snp_grouped}
\end{figure*}

%------------------------------------------------------------%
% -----------Uniform Noise: Loss Curves----------------------%
%------------------------------------------------------------%

\begin{figure*}[t]
    \centering

    \begin{subfigure}[t]{0.9\linewidth}
        \centering
        \includegraphics[width=\linewidth]{PaperSection/Pictures/PlotsAndGraphs/UniformNoise/LossCurves_UniformNoise_0.pdf}
        \caption{Angle-space noise $\sigma = 0$}
        \label{fig:loss_unif_sigma_0}
    \end{subfigure}
    \hfill
    \begin{subfigure}[t]{0.9\linewidth}
        \centering
        \includegraphics[width=\linewidth]{PaperSection/Pictures/PlotsAndGraphs/UniformNoise/LossCurves_UniformNoise_0.01.pdf}
        \caption{Angle-space noise $\sigma = 0.01$}
        \label{fig:loss_unif_sigma_001}
    \end{subfigure}

    \vspace{0.6em}

    \begin{subfigure}[t]{0.9\linewidth}
        \centering
        \includegraphics[width=\linewidth]{PaperSection/Pictures/PlotsAndGraphs/UniformNoise/LossCurves_UniformNoise_0.01.pdf}
        \caption{Angle-space noise $\sigma = 0.03$}
        \label{fig:loss_unif_sigma_003}
    \end{subfigure}
    \hfill
    \begin{subfigure}[t]{0.9\linewidth}
        \centering
        \includegraphics[width=\linewidth]{PaperSection/Pictures/PlotsAndGraphs/UniformNoise/LossCurves_UniformNoise_0.05.pdf}
        \caption{Angle-space noise $\sigma = 0.05$}
        \label{fig:loss_unif_sigma_005}
    \end{subfigure}

    \caption{Loss convergence curves for all circuit-level noise configurations under \textbf{uniform dataset noise}, shown for increasing angle-space noise magnitudes.}
    \label{fig:loss_unif_grouped}
\end{figure*}
%------------------------------------------------------------%
% -----------Uniform Noise: Accuracy Plots-------------------%
%------------------------------------------------------------%

\begin{figure*}[t]
    \centering

    \begin{subfigure}[t]{0.9\linewidth}
        \centering
        \includegraphics[width=0.8\linewidth]{PaperSection/Pictures/PlotsAndGraphs/UniformNoise/AccuracyBars_UniformNoise_0.pdf}
        \caption{Angle-space noise $\sigma = 0$}
        \label{fig:acc_unif_sigma_0}
    \end{subfigure}
    \hfill
    \begin{subfigure}[t]{0.9\linewidth}
        \centering
        \includegraphics[width=0.8\linewidth]{PaperSection/Pictures/PlotsAndGraphs/UniformNoise/AccuracyBars_UniformNoise_0.01.pdf}
        \caption{Angle-space noise $\sigma = 0.01$}
        \label{fig:acc_unif_sigma_001}
    \end{subfigure}

    \vspace{0.6em}

    \begin{subfigure}[t]{0.9\linewidth}
        \centering
        \includegraphics[width=0.8\linewidth]{PaperSection/Pictures/PlotsAndGraphs/UniformNoise/AccuracyBars_UniformNoise_0.03.pdf}
        \caption{Angle-space noise $\sigma = 0.03$}
        \label{fig:acc_unif_sigma_003}
    \end{subfigure}
    \hfill
    \begin{subfigure}[t]{0.9\linewidth}
        \centering
        \includegraphics[width=0.8\linewidth]{PaperSection/Pictures/PlotsAndGraphs/UniformNoise/AccuracyBars_UniformNoise_0.05.pdf}
        \caption{Angle-space noise $\sigma = 0.05$}
        \label{fig:acc_unif_sigma_005}
    \end{subfigure}

    \caption{Training and testing accuracy comparison for all circuit-level noise configurations under \textbf{uniform dataset noise}, shown for increasing angle-space perturbations.}
    \label{fig:acc_unif_grouped}
\end{figure*}

%------------------------------------------------------------%
% -----------speckle Noise: Loss Curves----------------------%
%------------------------------------------------------------%

\begin{figure*}[t]
    \centering

    \begin{subfigure}[t]{0.9\linewidth}
        \centering
        \includegraphics[width=\linewidth]{PaperSection/Pictures/PlotsAndGraphs/SpeckleNoise/LossCurves_SpeckleNoise_0.pdf}
        \caption{Angle-space noise $\sigma = 0$}
        \label{fig:loss_spec_sigma_0}
    \end{subfigure}
    \hfill
    \begin{subfigure}[t]{0.9\linewidth}
        \centering
        \includegraphics[width=\linewidth]{PaperSection/Pictures/PlotsAndGraphs/SpeckleNoise/LossCurves_SpeckleNoise_0.01.pdf}
        \caption{Angle-space noise $\sigma = 0.01$}
        \label{fig:loss_spec_sigma_001}
    \end{subfigure}

    \vspace{0.6em}

    \begin{subfigure}[t]{0.9\linewidth}
        \centering
        \includegraphics[width=\linewidth]{PaperSection/Pictures/PlotsAndGraphs/SpeckleNoise/LossCurves_SpeckleNoise_0.03.pdf}
        \caption{Angle-space noise $\sigma = 0.03$}
        \label{fig:loss_spec_sigma_003}
    \end{subfigure}
    \hfill
    \begin{subfigure}[t]{0.9\linewidth}
        \centering
        \includegraphics[width=\linewidth]{PaperSection/Pictures/PlotsAndGraphs/SpeckleNoise/LossCurves_SpeckleNoise_0.05.pdf}
        \caption{Angle-space noise $\sigma = 0.05$}
        \label{fig:loss_spec_sigma_005}
    \end{subfigure}

    \caption{Loss convergence curves for all circuit-level noise configurations under \textbf{Speckle noise}, shown for increasing angle-space noise magnitudes.}
    \label{fig:loss_spec_grouped}
\end{figure*}
%------------------------------------------------------------%
% -----------speckle Noise: Accuracy Plots-------------------%
%------------------------------------------------------------%

\begin{figure*}[t]
    \centering

    \begin{subfigure}[t]{0.9\linewidth}
        \centering
        \includegraphics[width=0.8\linewidth]{PaperSection/Pictures/PlotsAndGraphs/SpeckleNoise/AccuracyBars_SpeckleNoise_0.pdf}
        \caption{Angle-space noise $\sigma = 0$}
        \label{fig:acc_spec_sigma_0}
    \end{subfigure}
    \hfill
    \begin{subfigure}[t]{0.9\linewidth}
        \centering
        \includegraphics[width=0.8\linewidth]{PaperSection/Pictures/PlotsAndGraphs/SpeckleNoise/AccuracyBars_SpeckleNoise_0.01.pdf}
        \caption{Angle-space noise $\sigma = 0.01$}
        \label{fig:acc_spec_sigma_001}
    \end{subfigure}

    \vspace{0.6em}

    \begin{subfigure}[t]{0.9\linewidth}
        \centering
        \includegraphics[width=0.8\linewidth]{PaperSection/Pictures/PlotsAndGraphs/SpeckleNoise/AccuracyBars_SpeckleNoise_0.03.pdf}
        \caption{Angle-space noise $\sigma = 0.03$}
        \label{fig:acc_spec_sigma_003}
    \end{subfigure}
    \hfill
    \begin{subfigure}[t]{0.9\linewidth}
        \centering
        \includegraphics[width=0.8\linewidth]{PaperSection/Pictures/PlotsAndGraphs/SpeckleNoise/AccuracyBars_SpeckleNoise_0.05.pdf}
        \caption{Angle-space noise $\sigma = 0.05$}
        \label{fig:acc_spec_sigma_005}
    \end{subfigure}

    \caption{Training and testing accuracy comparison for all circuit-level noise configurations under \textbf{Speckle noise}, shown for increasing angle-space perturbations.}
    \label{fig:acc_spec_grouped}
\end{figure*}

%------------------------------------------------------------%
% -----------FeatureDropoutNoise: Loss Curves----------------------%
%------------------------------------------------------------%

\begin{figure*}[t]
    \centering

    \begin{subfigure}[t]{0.9\linewidth}
        \centering
        \includegraphics[width=\linewidth]{PaperSection/Pictures/PlotsAndGraphs/FeatureDropoutNoise/LossCurves_FeatureDropoutNoise_0.pdf}
        \caption{Angle-space noise $\sigma = 0$}
        \label{fig:loss_FD_sigma_0}
    \end{subfigure}
    \hfill
    \begin{subfigure}[t]{0.9\linewidth}
        \centering
        \includegraphics[width=\linewidth]{PaperSection/Pictures/PlotsAndGraphs/FeatureDropoutNoise/LossCurves_FeatureDropoutNoise_0.01.pdf}
        \caption{Angle-space noise $\sigma = 0.01$}
        \label{fig:loss_FD_sigma_001}
    \end{subfigure}
    \vspace{0.6em}

    \begin{subfigure}[t]{0.9\linewidth}
        \centering
        \includegraphics[width=\linewidth]{PaperSection/Pictures/PlotsAndGraphs/FeatureDropoutNoise/LossCurves_FeatureDropoutNoise_0.03.pdf}
        \caption{Angle-space noise $\sigma = 0.03$}
        \label{fig:loss_FD_sigma_003}
    \end{subfigure}
    \hfill
    \begin{subfigure}[t]{0.9\linewidth}
        \centering
        \includegraphics[width=\linewidth]{PaperSection/Pictures/PlotsAndGraphs/FeatureDropoutNoise/LossCurves_FeatureDropoutNoise_0.05.pdf}
        \caption{Angle-space noise $\sigma = 0.05$}
        \label{fig:loss_FD_sigma_005}
    \end{subfigure}

    \caption{Loss convergence curves for all circuit-level noise configurations under \textbf{Feature Dropout noise}, shown for increasing angle-space noise magnitudes.}
    \label{fig:loss_FD_grouped}
\end{figure*}
%------------------------------------------------------------%
% -----------Feature Dropout Noise: Accuracy Plots-------------------%
%------------------------------------------------------------%

\begin{figure*}[t]
    \centering

    \begin{subfigure}[t]{0.9\linewidth}
        \centering
        \includegraphics[width=0.8\linewidth]{PaperSection/Pictures/PlotsAndGraphs/FeatureDropoutNoise/AccuracyBars_FeatureDropoutNoise_0.pdf}
        \caption{Angle-space noise $\sigma = 0$}
        \label{fig:acc_FD_sigma_0}
    \end{subfigure}
    \hfill
    \begin{subfigure}[t]{0.9\linewidth}
        \centering
        \includegraphics[width=0.8\linewidth]{PaperSection/Pictures/PlotsAndGraphs/FeatureDropoutNoise/AccuracyBars_FeatureDropoutNoise_0.01.pdf}
        \caption{Angle-space noise $\sigma = 0.01$}
        \label{fig:acc_FD_sigma_001}
    \end{subfigure}

    \vspace{0.6em}

    \begin{subfigure}[t]{0.9\linewidth}
        \centering
        \includegraphics[width=0.8\linewidth]{PaperSection/Pictures/PlotsAndGraphs/FeatureDropoutNoise/AccuracyBars_FeatureDropoutNoise_0.03.pdf}
        \caption{Angle-space noise $\sigma = 0.03$}
        \label{fig:acc_FD_sigma_003}
    \end{subfigure}
    \hfill
    \begin{subfigure}[t]{0.9\linewidth}
        \centering
        \includegraphics[width=0.8\linewidth]{PaperSection/Pictures/PlotsAndGraphs/FeatureDropoutNoise/AccuracyBars_FeatureDropoutNoise_0.05.pdf}
        \caption{Angle-space noise $\sigma = 0.05$}
        \label{fig:acc_FD_sigma_005}
    \end{subfigure}

    \caption{Training and testing accuracy comparison for all circuit-level noise configurations under \textbf{Feature Dropout noise}, shown for increasing angle-space perturbations.}
    \label{fig:acc_FD_grouped}
\end{figure*}

%------------------------------------------------------------%
% -----------Quantization Noise: Loss Curves----------------------%
%------------------------------------------------------------%

\begin{figure*}[t]
    \centering

    \begin{subfigure}[t]{0.9\linewidth}
        \centering
        \includegraphics[width=\linewidth]{PaperSection/Pictures/PlotsAndGraphs/QuantizationNoise/LossCurves_QuantizationNoise_0.pdf}
        \caption{Angle-space noise $\sigma = 0$}
        \label{fig:loss_Quant_sigma_0}
    \end{subfigure}
    \hfill
    \begin{subfigure}[t]{0.9\linewidth}
        \centering
        \includegraphics[width=\linewidth]{PaperSection/Pictures/PlotsAndGraphs/QuantizationNoise/LossCurves_QuantizationNoise_0.01.pdf}
        \caption{Angle-space noise $\sigma = 0.01$}
        \label{fig:loss_Quant_sigma_001}
    \end{subfigure}
    \vspace{0.6em}

    \begin{subfigure}[t]{0.9\linewidth}
        \centering
        \includegraphics[width=\linewidth]{PaperSection/Pictures/PlotsAndGraphs/QuantizationNoise/LossCurves_QuantizationNoise_0.03.pdf}
        \caption{Angle-space noise $\sigma = 0.03$}
        \label{fig:loss_Quant_sigma_003}
    \end{subfigure}
    \hfill
    \begin{subfigure}[t]{0.9\linewidth}
        \centering
        \includegraphics[width=\linewidth]{PaperSection/Pictures/PlotsAndGraphs/QuantizationNoise/LossCurves_QuantizationNoise_0.05.pdf}
        \caption{Angle-space noise $\sigma = 0.05$}
        \label{fig:loss_Quant_sigma_005}
    \end{subfigure}

    \caption{Loss convergence curves for all circuit-level noise configurations under \textbf{Quantization noise}, shown for increasing angle-space noise magnitudes.}
    \label{fig:loss_Quant_grouped}
\end{figure*}
%------------------------------------------------------------%
% -----------Quantization Noise: Accuracy Plots-------------------%
%------------------------------------------------------------%

\begin{figure*}[t]
    \centering

    \begin{subfigure}[t]{0.9\linewidth}
        \centering
        \includegraphics[width=0.8\linewidth]{PaperSection/Pictures/PlotsAndGraphs/QuantizationNoise/AccuracyBars_QuantizationNoise_0.pdf}
        \caption{Angle-space noise $\sigma = 0$}
        \label{fig:acc_Quant_sigma_0}
    \end{subfigure}
    \hfill
    \begin{subfigure}[t]{0.9\linewidth}
        \centering
        \includegraphics[width=0.8\linewidth]{PaperSection/Pictures/PlotsAndGraphs/QuantizationNoise/AccuracyBars_QuantizationNoise_0.01.pdf}
        \caption{Angle-space noise $\sigma = 0.01$}
        \label{fig:acc_Quant_sigma_001}
    \end{subfigure}

    \vspace{0.6em}

    \begin{subfigure}[t]{0.9\linewidth}
        \centering
        \includegraphics[width=0.8\linewidth]{PaperSection/Pictures/PlotsAndGraphs/QuantizationNoise/AccuracyBars_QuantizationNoise_0.03.pdf}
        \caption{Angle-space noise $\sigma = 0.03$}
        \label{fig:acc_Quant_sigma_003}
    \end{subfigure}
    \hfill
    \begin{subfigure}[t]{0.9\linewidth}
        \centering
        \includegraphics[width=0.8\linewidth]{PaperSection/Pictures/PlotsAndGraphs/QuantizationNoise/AccuracyBars_QuantizationNoise_0.05.pdf}
        \caption{Angle-space noise $\sigma = 0.05$}
        \label{fig:acc_Quant_sigma_005}
    \end{subfigure}

    \caption{Training and testing accuracy comparison for all circuit-level noise configurations under \textbf{Quantization noise}, shown for increasing angle-space perturbations.}
    \label{fig:acc_Quant_grouped}
\end{figure*}

%------------------------------------------------------------%
% -----------Random Noise: Loss Curves----------------------%
%------------------------------------------------------------%

\begin{figure*}[t]
    \centering

    \begin{subfigure}[t]{0.9\linewidth}
        \centering
        \includegraphics[width=\linewidth]{PaperSection/Pictures/PlotsAndGraphs/RandomNoise/LossCurves_RandomNoise_0.pdf}
        \caption{Angle-space noise $\sigma = 0$}
        \label{fig:loss_Random_sigma_0}
    \end{subfigure}
    \hfill
    \begin{subfigure}[t]{0.9\linewidth}
        \centering
        \includegraphics[width=\linewidth]{PaperSection/Pictures/PlotsAndGraphs/RandomNoise/LossCurves_RandomNoise_0.01.pdf}
        \caption{Angle-space noise $\sigma = 0.01$}
        \label{fig:loss_Random_sigma_001}
    \end{subfigure}
    \vspace{0.6em}

    \begin{subfigure}[t]{0.9\linewidth}
        \centering
        \includegraphics[width=\linewidth]{PaperSection/Pictures/PlotsAndGraphs/RandomNoise/LossCurves_RandomNoise_0.03.pdf}
        \caption{Angle-space noise $\sigma = 0.03$}
        \label{fig:loss_Random_sigma_003}
    \end{subfigure}
    \hfill
    \begin{subfigure}[t]{0.9\linewidth}
        \centering
        \includegraphics[width=\linewidth]{PaperSection/Pictures/PlotsAndGraphs/RandomNoise/LossCurves_RandomNoise_0.05.pdf}
        \caption{Angle-space noise $\sigma = 0.05$}
        \label{fig:loss_Random_sigma_005}
    \end{subfigure}

    \caption{Loss convergence curves for all circuit-level noise configurations under \textbf{Random noise}, shown for increasing angle-space noise magnitudes.}
    \label{fig:loss_Random_grouped}
\end{figure*}
%------------------------------------------------------------%
% -----------Random Noise: Accuracy Plots-------------------%
%------------------------------------------------------------%

\begin{figure*}[t]
    \centering

    \begin{subfigure}[t]{0.9\linewidth}
        \centering
        \includegraphics[width=0.8\linewidth]{PaperSection/Pictures/PlotsAndGraphs/RandomNoise/AccuracyBars_RandomNoise_0.pdf}
        \caption{Angle-space noise $\sigma = 0$}
        \label{fig:acc_Random_sigma_0}
    \end{subfigure}
    \hfill
    \begin{subfigure}[t]{0.9\linewidth}
        \centering
        \includegraphics[width=0.8\linewidth]{PaperSection/Pictures/PlotsAndGraphs/RandomNoise/AccuracyBars_RandomNoise_0.01.pdf}
        \caption{Angle-space noise $\sigma = 0.01$}
        \label{fig:acc_Random_sigma_001}
    \end{subfigure}

    \vspace{0.6em}

    \begin{subfigure}[t]{0.9\linewidth}
        \centering
        \includegraphics[width=0.8\linewidth]{PaperSection/Pictures/PlotsAndGraphs/RandomNoise/AccuracyBars_RandomNoise_0.03.pdf}
        \caption{Angle-space noise $\sigma = 0.03$}
        \label{fig:acc_Random_sigma_003}
    \end{subfigure}
    \hfill
    \begin{subfigure}[t]{0.9\linewidth}
        \centering
        \includegraphics[width=0.8\linewidth]{PaperSection/Pictures/PlotsAndGraphs/RandomNoise/AccuracyBars_RandomNoise_0.05.pdf}
        \caption{Angle-space noise $\sigma = 0.05$}
        \label{fig:acc_Random_sigma_005}
    \end{subfigure}

    \caption{Training and testing accuracy comparison for all circuit-level noise configurations under \textbf{Random noise}, shown for increasing angle-space perturbations.}
    \label{fig:acc_Random_grouped}
\end{figure*}

These comprehensive visualizations corroborate the trends discussed in the main text, demonstrating abrupt optimization collapse under circuit-level quantum noise, gradual degradation under coherent angle-space perturbations, and comparatively weaker sensitivity to dataset-level noise in the absence of hardware noise.
\end{appendix}
